# Supplementary material for: Towards Robust Deep Learning with Ensemble Networks and Noisy Layers
Source: arXiv:2007.01507 source file (2021-01-06)
Supplement: Supplementary file 1 [file Appendix.tex]

\appendix
\section*{Appendix}
\label{appendix}

\subsection{Superimposition Attack using $L_\infty$ Norm}
\label{SI3_Linfinity}
In this section we present the results from applying the Superimposition ($3\times$) attack with the $L_\infty$ norm to our model. In Table \ref{tab:distribution_clean_vs_super3_Li} we observe similarly that Noisy Logit reduces the success rate of attack on the individual networks and Ensemble Voting allows accuracy to be further improved for both datasets.

    \begin{table}[]
 \centering
%  \begin{multicols}{3}
 %  \hspace{-0.9cm}
\begin{subtable}{1.0\linewidth} 
\centering
\subcaption{Average accuracy}
\vspace{-0.2cm} 
    \resizebox{0.95\textwidth}{!}{%
    \begin{tabular}{@{}lll@{}}
    \toprule
    \textbf{Single Network}  & \textbf{Clean Accuracy} & \textbf{SI3 Attack Accuracy}  \\ \midrule
MNIST Network                    & 95.60\%        & 19.13\%             \\
MNIST Network with Noisy Logit   & 75.22\%        & 49.07\%             \\
CIFAR10 Network                  & 83.00\%        & 68.53\%             \\
CIFAR10 Network with Noisy Logit & 77.47\%        & 68.22\%             \\ \bottomrule
    \end{tabular}%
    }  
\label{tab:accuracy_clean_vs_super3_Li}
    \end{subtable}  
% \columnbreak
% \hspace{-0.9cm}

\vspace{0.25cm} 
\begin{subtable}{1.0\linewidth} 
\centering
\subcaption{Classifications}
\vspace{-0.2cm}  
    \resizebox{0.95\textwidth}{!}{%
        \begin{tabular}{@{}llll@{}}
        \toprule
        \textbf{Model}        & \textbf{Correct} & \textbf{Target} & \textbf{Other}     \\ \midrule
MNIST Ensemble                    & 18.89\% & 64.44\% & 16.67\% \\
MNIST Ensemble with Noisy Logit   & 76.67\% & 12.22\% & 11.11\% \\
CIFAR10 Ensemble                  & 85.56\% & 1.11\%  & 13.33\% \\
CIFAR10 Ensemble with Noisy Logit & 87.78\% & 1.11\%  & 11.11\% \\ \bottomrule
        \end{tabular}%
        }    
    \label{tab:classification_clean_vs_super3_Li}
        \end{subtable}

%\columnbreak
% \hspace{-0.9cm}
\vspace{0.25cm} 
\begin{subtable}{1.0\linewidth} 
\centering
\subcaption{Average perturbations}
\vspace{-0.2cm} 
    \resizebox{0.95\textwidth}{!}{%
            \begin{tabular}{@{}llll@{}}
            \toprule
            \textbf{Model} & \textbf{Correct} & \textbf{Target} & \textbf{Other} \\ \midrule
MNIST Ensemble                    & 11.78\% & 39.37\% & 49.01\% \\
MNIST Ensemble with Noisy Logit   & 10.08\% & 46.62\% & 28.07\% \\
CIFAR10 Ensemble                  & 5.42\%  & 0.00\%  & 8.09\%  \\
CIFAR10 Ensemble with Noisy Logit & 5.41\%  & 0.00\%  & 4.99\%  \\ \bottomrule
            \end{tabular}%
            }       
            \label{tab:perturb_clean_vs_super3_Li}
            \end{subtable}
 %\end{multicols}
 
 \vspace{0.3cm}    
            \caption{Distributions for Superimposition ($3\times$) of adversarial inputs. (a) average single network clean accuracy vs. attack accuracy; (b) breakdown of classifications; (c) average perturbations corresponding to classifications.} 
        \label{tab:distribution_clean_vs_super3_Li}
            \end{table}

\subsection{A Second Look at Noisy Logit}
\label{detailed_noisylogit}
The results for the Random Single Network Attack in Section~\ref{SN_results} provided some insights into how Noisy Logit works to reduce transferability across different neural networks. However, in the case of the MNIST dataset, we observed that although Noisy Logit changes the distribution of perturbations in the adversarial examples, it appears there is no benefit to using Noisy Logit as Ensemble Voting alone provides better accuracy rates. In this section, we look at the output of each individual network in isolation when it's being targeted, to see whether applying Noisy Logit improves robustness in a single network. In Fig.~\ref{fig:adversarial_examples_withandwithout_noisylogit} we craft adversarial examples corresponding to a single sample and single target, on each of the 50 networks in the ensemble.

\begin{figure}[!t]
\centering
\begin{minipage}{0.47\textwidth}
\begin{subfigure}{0.47\textwidth}
    %\begin{minipage}{0.38\textwidth}
 \subcaption{\footnotesize MNIST No Noisy Logit}
 \label{fig:mnist_input0_target0_all}
 \vspace {-.05cm}   
  \includegraphics[width=1\textwidth]{Plots/mnist/input0_target0_all.png}
  %\end{minipage}
    \end{subfigure} 
  \hfill
\begin{subfigure}{0.47\textwidth}
\subcaption{\footnotesize MNIST With Noisy Logit}
\label{fig:mnist_input0_target0_noisy}
\vspace {-.05cm}
    %\begin{minipage}{0.38\textwidth}
\includegraphics[width=1\textwidth]{Plots/mnist/input0_target0_noisy.png}
    \end{subfigure} 
\end{minipage}
%\vspace {.2cm}
\vfill

\begin{minipage}{0.47\textwidth}
\begin{subfigure}{0.47\textwidth}
\subcaption{\footnotesize CIFAR10 No Noisy Logit}
\label{fig:CIFAR10_input0_target0_all}
\vspace {-.05cm}
    %\begin{minipage}{0.38\textwidth}
  \includegraphics[width=1\textwidth]{Plots/cifar/input0_target0_all.png}
    %\end{minipage}
    \end{subfigure} 
  \hfill
\begin{subfigure}{0.47\textwidth}
\subcaption{\footnotesize CIFAR10 With Noisy Logit}
\label{fig:CIFAR10_input0_target0_noisy}
\vspace {-.05cm}
    %\begin{minipage}{0.38\textwidth}
\includegraphics[width=1\textwidth]{Plots/cifar/input0_target0_noisy.png}
    \end{subfigure}
\end{minipage}
%\vspace {-.05cm}
    \caption{Adversarial examples without and with Noisy Logit applied}
    \label{fig:adversarial_examples_withandwithout_noisylogit} 
    \end{figure}

\begin{table}[]
\begin{subtable}{0.45\linewidth} 
\centering
\subcaption{MNIST}
\vspace{-0.2cm} 
\begin{tabular}{|l|l|l|l|l|}
\hline
7 & 7 & 7 & 5 & 0 \\ \hline
7 & 0 & 7 & 0 & 2 \\ \hline
7 & 7 & 7 & 7 & 7 \\ \hline
7 & 0 & 7 & 0 & 2 \\ \hline
7 & 7 & 3 & 2 & 2 \\ \hline
7 & 7 & 3 & 7 & 7 \\ \hline
2 & 7 & 7 & 7 & 3 \\ \hline
7 & 7 & 7 & 2 & 0 \\ \hline
3 & 7 & 5 & 0 & 7 \\ \hline
7 & 2 & 7 & 0 & 7 \\ \hline
\end{tabular}
\label{tab:class_input7target0_noisy_mnist}
\end{subtable}
\vspace{0.3cm}
\begin{subtable}{0.45\linewidth} 
\centering
\subcaption{CIFAR10}
\vspace{-0.2cm}
\begin{tabular}{|l|l|l|l|l|}
\hline
8 & 8 & 1 & 8 & 8 \\ \hline
8 & 8 & 1 & 8 & 8 \\ \hline
8 & 8 & 1 & 8 & 8 \\ \hline
8 & 8 & 8 & 8 & 1 \\ \hline
8 & 1 & 8 & 8 & 8 \\ \hline
8 & 1 & 1 & 8 & 8 \\ \hline
8 & 8 & 8 & 8 & 0 \\ \hline
8 & 8 & 8 & 8 & 1 \\ \hline
1 & 1 & 8 & 8 & 8 \\ \hline
1 & 8 & 8 & 8 & 8 \\ \hline
\end{tabular}
\label{tab:class_input7target0_noisy_cifar}
\end{subtable} 
\caption{Classifications of the 50 networks corresponding to Fig. \ref{fig:mnist_input0_target0_noisy} and Fig. \ref{fig:CIFAR10_input0_target0_noisy}, respectively. In (a), the numbered classifications correspond to the digits; in (b), 8 corresponds to ship, 1 corresponds to automobile and 0 corresponds to airplane.}
\label{tab:classification_input7target0_noisy}
\end{table}

In Fig.~\ref{fig:mnist_input0_target0_all} and Fig.~\ref{fig:mnist_input0_target0_noisy}, the sample input is the digit 7 and target is the digit 0. Observe that the distribution of perturbations is changed if we apply Noisy Logit, where in Fig.~\ref{fig:mnist_input0_target0_noisy} we see more occurrences in the tails (i.e. very small or very large perturbations). In Fig.~\ref{fig:mnist_input0_target0_all} each targeted network mis-classifies its corresponding adversarial example as 0 (corresponding to $100\%$ success rate of Carlini-Wagner on a single network); whereas in Fig.~\ref{fig:mnist_input0_target0_noisy}, only 8 of the networks misclassify as 0, and 29 of the networks still correctly classify as 7 as shown in Table \ref{tab:class_input7target0_noisy_mnist}. Therefore, for an individual MNIST network with Noisy Logit applied, the success rate of a targeted Carlni-Wagner attack is low. Thus, a single MNIST network is more robust to adversarial examples if Noisy Logit is applied, however the accuracy rate suffers since extra noise is added.

In Fig.~\ref{fig:CIFAR10_input0_target0_all} and Fig.~\ref{fig:CIFAR10_input0_target0_noisy}, the sample input is the object ship and the target is the object airplane. There is no noticeable difference in the distribution of perturbations whether or not Noisy Logit is applied. In Fig.~\ref{fig:CIFAR10_input0_target0_all}, again each targeted network misclassifies its corresponding adversarial example as the target (airplane); whereas in Fig.~\ref{fig:CIFAR10_input0_target0_noisy}, only 1 of the networks misclassifies as airplane, and 38 of the networks still correctly classify as ship as shown in Table \ref{tab:class_input7target0_noisy_cifar}. Therefore, the success rate of a targeted Carlni-Wagner attack on a single CIFAR10 network is very low, i.e., robustness of a single CIFAR10 network is increased in the presence of Noisy Logit. Note also the accuracy rate only slightly suffers from extra noise added. 
%We provide the actual classifications corresponding to Fig. \ref{fig:mnist_input0_target0_noisy} and Fig. \ref{fig:CIFAR10_input0_target0_noisy} in Table \ref{tab:classification_input7target0_noisy}.

\subsection{Sample Results for Superimposition Attacks}
In Fig. \ref{fig:mnist_sup2_simple_sample1} - Fig. \ref{fig:cifar_sup3_noisy_sample2} samples of resulting images with adversarial perturbations are shown. The leftmost column displays the original images, the middle columns display the adversarial examples with the two or three smallest perturbations, the last column shows the superimposition of the two or three adversarial examples. The rows correspond to different targets being applied in the adversarial examples. Classifications of these images are provided in Tables \ref{tab:mnist_classifications_sample1} - \ref{tab:cifar_classifications_sample2}. 

\begin{figure}[t]
   \begin{minipage}{0.47\textwidth}
\begin{subfigure}{0.47\textwidth}
    \subcaption{Without Noisy Logit ($2\times$)}
    \vspace {-.05cm}
  \includegraphics[width=1\textwidth]{Plots/mnist/sup2_simple_sample1.png}  
          \label{fig:mnist_sup2_simple_sample1}
  %\end{minipage}
    \end{subfigure} 
  \hfill
\begin{subfigure}{0.47\textwidth}
    %\begin{minipage}{0.22\textwidth}
    \subcaption{With Noisy Logit ($2\times$)}
    \vspace {-.05cm}
\includegraphics[width=1\textwidth]{Plots/mnist/sup2_noisy_sample1.png}
        \label{fig:mnist_sup2_noisy_sample1}
    \end{subfigure}
    \end{minipage} 

      \begin{minipage}{0.47\textwidth}
	\begin{subfigure}{0.47\textwidth}
        \subcaption{Without Noisy Logit ($3\times$)}
        \vspace {-.05cm}
      \includegraphics[width=1\textwidth]{Plots/mnist/sup3_simple_sample1.png}
              \label{fig:mnist_sup3_simple_sample1}
      %\end{minipage}
    \end{subfigure} 
  \hfill
\begin{subfigure}{0.47\textwidth}
        %\begin{minipage}{0.22\textwidth}
         \subcaption{With Noisy Logit ($3\times$)}
         \vspace {-.05cm}
    \includegraphics[width=1\textwidth]{Plots/mnist/sup3_noisy_sample1.png}
            \label{fig:mnist_sup3_noisy_sample1}
       \end{subfigure}
        \end{minipage} 
        \vspace {-.3cm}
        \caption{Adversarial Images using Superimposition ($2\times$ and $3\times$) MNIST Sample 1}
        \end{figure}

\begin{table}[]
\resizebox{0.44\textwidth}{!}{%
\begin{tabular}{@{}lllll@{}}
\toprule
Target & SI ($2\times$) & SI-NL ($2\times$) & SI ($3\times$) & SI-NL ($3\times$) \\ \midrule
0      & 7       & 7          & 0       & 7          \\
1      & 2       & 7          & 2       & 7          \\
2      & 7       & 7          & 2       & 7          \\
3      & 7       & 7          & 3       & 7          \\
4      & 4       & 7          & 4       & 7          \\
5      & 7       & 7          & 5       & 7          \\
6      & 6       & 7          & 6       & 7          \\
8      & 7       & 7          & 8       & 7          \\
9      & 9       & 7          & 9       & 7          \\ \bottomrule
\end{tabular}%
}
\caption{Classifications of MNIST Sample 1, corresponding to Fig. \ref{fig:mnist_sup2_simple_sample1}, \ref{fig:mnist_sup2_noisy_sample1}, \ref{fig:mnist_sup3_simple_sample1}, \ref{fig:mnist_sup3_noisy_sample1}, respectively.}
\label{tab:mnist_classifications_sample1}
\end{table}

\begin{figure}[!t]
       \begin{minipage}{0.47\textwidth}
\begin{subfigure}{0.47\textwidth}
   \subcaption{Without Noisy Logit ($2\times$)}
    \vspace {-.05cm}
  \includegraphics[width=1\textwidth]{Plots/mnist/sup2_simple_sample2.png}
          \label{fig:mnist_sup2_simple_sample2}
  %\end{minipage}
  \end{subfigure}
  \hfill
    %\begin{minipage}{0.22\textwidth}
    \begin{subfigure}{0.47\textwidth}
    \subcaption{With Noisy Logit ($2\times$)}
    \vspace {-.05cm}
\includegraphics[width=1\textwidth]{Plots/mnist/sup2_noisy_sample2.png}
        \label{fig:mnist_sup2_noisy_sample2}
    \end{subfigure}    
    \end{minipage} 

     \begin{minipage}{0.47\textwidth}
	\begin{subfigure}{0.47\textwidth}
        \subcaption{Without Noisy Logit ($3\times$)}
        \vspace {-.05cm}
      \includegraphics[width=1\textwidth]{Plots/mnist/sup3_simple_sample2.png}
              \label{fig:mnist_sup3_simple_sample2}
     \end{subfigure}
      %\end{minipage}
      \hfill
        %\begin{minipage}{0.22\textwidth}
      \begin{subfigure}{0.47\textwidth}
        \subcaption{With Noisy Logit ($3\times$)}
        \vspace {-.05cm}
    \includegraphics[width=1\textwidth]{Plots/mnist/sup3_noisy_sample2.png}
            \label{fig:mnist_sup3_noisy_sample2}
        \end{subfigure}    
        \end{minipage} 
        \vspace {-.3cm}
        \caption{Adversarial Images using Superimposition ($2\times$ and $3\times$) MNIST Sample 2}
        \end{figure}        

\begin{table}[]
\resizebox{0.44\textwidth}{!}{%
\begin{tabular}{@{}lllll@{}}
\toprule
Target & SI ($2\times$) & SI-NL ($2\times$) & SI ($3\times$) & SI-NL ($3\times$) \\ \midrule
0      & 2       & 2          & 2       & 2          \\
1      & 2       & 2          & 2       & 2          \\
3      & 2       & 2          & 3       & 2          \\
4      & 8       & 2          & 4       & 4          \\
5      & 2       & 2          & 5       & 2          \\
6      & 2       & 2          & 6       & 2          \\
7      & 7       & 8          & 7       & 3          \\
8      & 2       & 2          & 8       & 2          \\
9      & 8       & 2          & 9       & 9          \\ \bottomrule
\end{tabular}%
}
\caption{Classifications of MNIST Sample 2, corresponding to Fig. \ref{fig:mnist_sup2_simple_sample2}, \ref{fig:mnist_sup2_noisy_sample2}, \ref{fig:mnist_sup3_simple_sample2}, \ref{fig:mnist_sup3_noisy_sample2}, respectively.}
\label{tab:mnist_classifications_sample2}
\end{table}

\begin{figure}[!t]
           \begin{minipage}{0.47\textwidth}
\begin{subfigure}{0.47\textwidth}
    \subcaption{Without Noisy Logit ($2\times$)}
    \vspace {-.05cm}
  \includegraphics[width=1\textwidth]{Plots/cifar/sup2_simple_sample1.png}   
          \label{fig:cifar_sup2_simple_sample1}
  %\end{minipage}
  \end{subfigure}
  \hfill
    %\begin{minipage}{0.22\textwidth}
   \begin{subfigure}{0.47\textwidth}
    \subcaption{With Noisy Logit ($2\times$)}
    \vspace {-.05cm}
\includegraphics[width=1\textwidth]{Plots/cifar/sup2_noisy_sample1.png}
        \label{fig:cifar_sup2_noisy_sample1}
   \end{subfigure}
   \end{minipage} 
    %\vspace {-.2cm}
    %\caption{Adversarial Images using Superimposition ($2\times$) CIFAR Sample 1}
    %\end{figure}

   %\begin{figure}[!t]
        %\begin{minipage}{0.22\textwidth}
   \begin{minipage}{0.47\textwidth}
\begin{subfigure}{0.47\textwidth}
       \subcaption{Without Noisy Logit ($3\times$)}
        \vspace {-.05cm}
      \includegraphics[width=1\textwidth]{Plots/cifar/sup3_simple_sample1.png}
         \label{fig:cifar_sup3_simple_sample1}
      \end{subfigure}
      %\end{minipage}
      \hfill
        %\begin{minipage}{0.22\textwidth}
       \begin{subfigure}{0.47\textwidth}
        \subcaption{With Noisy Logit ($3\times$)}
        \vspace {-.05cm}
    \includegraphics[width=1\textwidth]{Plots/cifar/sup3_noisy_sample1.png}
            \label{fig:cifar_sup3_noisy_sample1}
        \end{subfigure}
        \end{minipage} 
        \vspace {-.3cm}
        \caption{Adversarial Images using Superimposition ($3\times$) CIFAR Sample 1}
        \end{figure}
        
\begin{table}[]
\resizebox{0.44\textwidth}{!}{%
\begin{tabular}{@{}lllll@{}}
\toprule
Target & SI ($2\times$) & SI-NL ($2\times$) & SI ($3\times$) & SI-NL ($3\times$) \\ \midrule
0      & 3       & 3          & 3       & 3          \\
1      & 3       & 3          & 3       & 3          \\
2      & 3       & 3          & 3       & 3          \\
4      & 3       & 3          & 3       & 3          \\
5      & 3       & 3          & 3       & 3          \\
6      & 3       & 3          & 3       & 3          \\
7      & 3       & 3          & 3       & 3          \\
8      & 3       & 3          & 3       & 3          \\
9      & 3       & 3          & 3       & 3          \\ \bottomrule
\end{tabular}%
}
\caption{Classifications of CIFAR Sample 1, corresponding to Fig. \ref{fig:cifar_sup2_simple_sample1}, \ref{fig:cifar_sup2_noisy_sample1}, \ref{fig:cifar_sup3_simple_sample1}, \ref{fig:cifar_sup3_noisy_sample1}, respectively.}
\label{tab:cifar_classifications_sample1}
\end{table}     

\begin{figure}[!t]
     \begin{minipage}{0.47\textwidth}
\begin{subfigure}{0.47\textwidth}
    \subcaption{Without Noisy Logit ($2\times$)}
    \vspace {-.05cm}
  \includegraphics[width=1\textwidth]{Plots/cifar/sup2_simple_sample2.png}
          \label{fig:cifar_sup2_simple_sample2}
  %\end{minipage}
  \end{subfigure}
  \hfill
    %\begin{minipage}{0.22\textwidth}
    \begin{subfigure}{0.47\textwidth}
    \subcaption{With Noisy Logit ($2\times$)}
    \vspace {-.05cm}
\includegraphics[width=1\textwidth]{Plots/cifar/sup2_noisy_sample2.png}
        \label{fig:cifar_sup2_noisy_sample2}
    \end{subfigure}
    \end{minipage} 
   % \vspace {-.3cm}
   % \caption{Adversarial Images using Superimposition ($2\times$) CIFAR Sample 2}
   % \end{figure}    

    %\begin{figure}[!t]
     %   \begin{minipage}{0.22\textwidth}
     \begin{minipage}{0.47\textwidth}
\begin{subfigure}{0.47\textwidth}
       \subcaption{Without Noisy Logit ($3\times$)}
        \vspace {-.05cm}
      \includegraphics[width=1\textwidth]{Plots/cifar/sup3_simple_sample2.png}
              \label{fig:cifar_sup3_simple_sample2}
       \end{subfigure}       
      %\end{minipage}
      \hfill
        %\begin{minipage}{0.22\textwidth}
        \begin{subfigure}{0.47\textwidth}
       \subcaption{With Noisy Logit ($3\times$)}
        \vspace {-.05cm}
    \includegraphics[width=1\textwidth]{Plots/cifar/sup3_noisy_sample2.png}  
            \label{fig:cifar_sup3_noisy_sample2}
        \end{subfigure}
        \end{minipage} 
        \vspace {-.3cm}
        \caption{Adversarial Images using Superimposition ($2\times$ and $3\times$) CIFAR Sample 2}
        \end{figure}    

\begin{table}[]
\resizebox{0.44\textwidth}{!}{%
\begin{tabular}{@{}lllll@{}}
\toprule
Target & SI ($2\times$) & SI-NL ($2\times$) & SI ($3\times$) & SI-NL ($3\times$) \\ \midrule
0      & 8       & 8          & 8       & 8          \\
1      & 8       & 8          & 8       & 8          \\
2      & 8       & 8          & 8       & 8          \\
3      & 8       & 8          & 8       & 8          \\
4      & 8       & 8          & 8       & 8          \\
5      & 8       & 8          & 8       & 1          \\
6      & 8       & 8          & 8       & 8          \\
7      & 8       & 8          & 0       & 8          \\
9      & 1       & 8          & 1       & 8          \\ \bottomrule
\end{tabular}%
}
\caption{Classifications of CIFAR Sample 2, corresponding to Fig. \ref{fig:cifar_sup2_simple_sample2}, \ref{fig:cifar_sup2_noisy_sample2}, \ref{fig:cifar_sup3_simple_sample2}, \ref{fig:cifar_sup3_noisy_sample2}, respectively.}
\label{tab:cifar_classifications_sample2}
\end{table}

%In Fig. \ref{fig:mnist_sup2_simple_sample1} - Fig. \ref{fig:cifar_sup3_noisy_sample2} samples of resulting images with adversarial perturbations are shown. The leftmost column displays the original images, the middle columns display the adversarial examples with the two or three smallest perturbations, the last column shows the superimposition of the two or three adversarial examples. The rows correspond to different targets being applied in the adversarial examples. Classifications of these images are provided in Tables \ref{tab:mnist_classifications_sample1} - \ref{tab:cifar_classifications_sample2}. 

%The images provided were generated from the superimposition attacks; the steps to generate these are provided in the attached source code and described in the README file.

% In Sample 1, using simple Ensemble Voting (Fig. \ref{fig:mnist_sup2_simple_sample1}), 3/9 of the superimposed images were mis-classified, whereas using Ensemble Voting with Noisy Logit (Fig. \ref{fig:mnist_sup2_noisy_sample1}) all of the superimposed images were still correctly classified. For Sample 2, the numbers are 4/9 and 1/9, respectively. Examining the samples, it appears that when the Noisy Logit mechanism is used, the same attack mechanism results in smaller perturbations for the MNIST dataset, and also that the Noisy Logit mechanism interferes with the ability of an attack mechanism to produce effective perturbations as some images with noticeable perturbations were still correctly classified by the combined network.
